# Supplementary material for: Transformer Networks for Trajectory Forecasting
Source: arXiv:2003.08111 source file (2020-10-21)
Supplement: Supplementary file 1 [file SuppMat.tex]

\newpage
\clearpage

\section{Supplementary material}

Here we paste the experiments which we have decided to not include into the paper, but ``may'' get into the supplementary material.

\todo{Include here the correct one table for the varying horizon, as the experiments\_old.tex file contains multiple versions.}

\begin{table}[b]
  \centering
  \caption{Mean Average Displacement (MAD) error when changing the observation interval. Forecasting horizon is kept constant at 12 frames. \todo{This table should probably be omitted.}}
  \label{table:table3Ab}
  \resizebox{\linewidth}{!}{
    \begin{tabular}{|l|l||l|l|}
    \hline
    Dataset & Prediction interval & Vanilla LSTM & Individual TF\\
    \hline \hline
    \multirow{3}{*}{\vspace{-1em}\textbf{Eth}} &
    \textbf{Obs = 8} & 0.61 / 1.20 & 0.62 / 1.24\\
    \cline{2-4}
    &\textbf{Obs = 12} & 0.58 / 1.16 & 0.65 / 1.31\\
    \cline{2-4}
    & \textbf{Obs = 16} & 0.59 / 1.18 & 0.65 / 1.25\\
    
    \hline \hline
    \multirow{3}{*}{\vspace{-1em}\textbf{Hotel}} &
    \textbf{Obs = 8} &  0.53 / 1.13 & 0.34 / 0.66\\
    \cline{2-4}
    & \textbf{Obs = 12} & 0.36 / 0.73 &  0.32 / 0.61\\
    \cline{2-4}
    & \textbf{Obs = 16} & 0.29 / 0.55 & 0.26 / 0.45\\
  
    \hline \hline
    \multirow{3}{*}{\vspace{-1em}\textbf{Uvy-univ}} &
    \textbf{Obs = 8} & 0.57 / 1.18 & 0.60 / 1.30\\
    \cline{2-4}
    &\textbf{Obs = 12} & 0.55 / 1.23 & 0.66 / 1.39\\
    \cline{2-4}
    & \textbf{Obs = 16} & 0.53 / 1.19 & 0.65 / 1.25  \\
    \cline{2-4}
    \hline \hline
    \multirow{3}{*}{\vspace{-1 em}\textbf{Zara1}} &
    \textbf{Obs = 8} & 0.42 / 0.92 & 0.42 / 0.92\\
    \cline{2-4}
    &\textbf{Obs = 12} & 0.41 / 0.91 & 0.43 / 0.95\\
    \cline{2-4}
    & \textbf{Obs = 16} & 0.41 / 0.92 & 0.47 / 1.05\\
    \cline{2-4}
    \hline \hline
    \multirow{4}{*}{\vspace{-1 em}\textbf{Zara2}} &
    \textbf{Obs = 8} & 0.35 / 0.78 & 0.34 / 0.74\\
    \cline{2-4}
    &\textbf{Obs = 12} & 0.32 / 0.72 & 0.38 / 0.85\\
    \cline{2-4}
    & \textbf{Obs = 16} & 0.29 / 0.68 & 0.30 / 0.67\\
    \cline{2-4}

     \hline
    \end{tabular}
  }
\end{table}

\begin{table*}[t!]
\caption{Results with Social GAN data-outdated}
  \centering
  \resizebox{0.9\linewidth}{!}{%
  \begin{tabular}{l|l|l|l|l|l|l|l|l|l|l|l|l}
    \midrule
    & \multicolumn{7}{c|}{\textbf{Baselines}} & \multicolumn{5}{c}{\textbf{Social Transformer (Ours)}} \\
    \cmidrule[1pt]{2-13}
    \textbf{Dataset} & \textbf{Lin} & \textbf{LSTM} & \textbf{S-LSTM} & \textbf{S-GAN} & \textbf{S-GAN-P} & \textbf{SoPhie} & \textbf{SR-LSTM} & \textbf{TK} & $\mathbf{Tk+ DA}$ & $\mathbf{Tk+OccMaps}$ & \textbf{TK(SR-LSTM dt)} &\textbf{TK+OCC(SR-LSTM dt)}\\
    \midrule
\textbf{ETH} & 1.33 / 2.94 & 1.09 / 2.41 & 1.09 / 2.35 & 0.81 / 1.52  & 0.87 /  1.62 & 0.70 / 1.43 &\textbf{0.63 / 1.25}& 1.07 / 2.22 & 1.02 / 2,18 & 0.83 / 1.74 & 0.65 & 0.66 / 1.40\\
    \textbf{HOTEL} & 0.39 / 0.72 & 0.86 / 1.91 & 0.79 / 1.76 &  0.72 / 1.61 & 0.67 / 1.37 & 0.76 / 1.67 &0.37 / 0.74& 0.53 / 1.15 & 0.3 / 0.58 & 0.33 / 0.71 &0.34 & \textbf{0.33/ 0.73}\\
    \textbf{UNIV}  & 0.82 /  1.59 &  0.61 /  1.31 & 0.67 / 1.40 & 0.60 / 1.26 & 0.76 / 1.52 & 0.54 / 1.24& 0.51 / 1.10 & na & 0.55 / 1.19 & 0.52 / 1.11 & 0.59 / 1.27 & \textbf{0.50 / 1.14}\\
    \textbf{ZARA1} & 0.62 / 1.21 & 0.41 / 0.88 & 0.47 / 1.00 & 0.34 / 0.69 & 0.35 / 0.68 & \textbf{0.30 / 0.63} &0.41 / 0.90  & 0.41 / 0.91 & 0.45 / 0.98 & 0.36 / 0.85 &0.40 & 0.32 / 0.75\\
    \textbf{ZARA2} & 0.77 / 1.48& 0.52 / 1.11 & 0.56 /  1.17&  0.42 / 0.84 & 0.42 / 0.84 & 0.38 / 0.78 & 0.32 / 0.70  & 0.31 / 0.69 & 0.33 / 0.73 & 0.26 / 0.64 & 0.31 & \textbf{0.25 / 0.57}\\
    \toprule
    \midrule
    \textbf{AVG}   & 0.79 / 1.59 & 0.70 /  1.52  & 0.72 / 1.54 & 0.58 / 1.18 & 0.61 / 1.21 & 0.54 / 1.15 & 0.45 / 0.94&na & 0.53 / 1.13  & 0.46 / 1.01 & 0.45& \textbf{0.41 / 0.91}\\
    \toprule
  \end{tabular}
  }
\end{table*}

\begin{table*}[]
\caption{Comparison with SOTA and MX-LSTM on Mx-LSTM data \todo{include the current results of TK+vislets}}
 \resizebox{0.9\linewidth}{!}{
\begin{tabular}{|l|l|l|l|l|l|l|l|l|}
\hline
Datasets & LTA \cite{pellegrini2009iccv}       & SF \cite{yamaguchi2011cvpr}        & Social LSTM \cite{alahi2016cvpr} & Social GAN \cite{SocialGAN18} & Indiv-Mx-LSTM \cite{Hasan18} & MX-LSTM \cite{Hasan18}   & TK         & TK + OCC \\ \hline
Univ     & 2.49/4.66 & 2.57/4.62 & 0.62/1.40   & 0.65/1.36  & 0.53/1.16     & 0.49/1.12 & 0.44//0.99 &          \\ \hline
Zara1    & 2.74/5.55 & 2.88/5.55 & 0.68/1.53   & 0.48/1.04  & 0.63/1.37     & 0.59/1.31 & 0.31/0.69  &          \\ \hline
Zara2    & 2.23/4.35 & 2.32/4.35 & 0.63/1.43   & 0.44/0.95  & 0.72/1.56     & 0.35/0.79 & 0.25/0.56  &          \\ \hline
\end{tabular}
}
\end{table*}

% \begin{table}[]
% \caption{Ablation study with MX-LSTM on Mx-LSTM data}
%  \resizebox{0.9\linewidth}{!}{
% \begin{tabular}{|l|l|l|l|l|}
% \hline
% Datasets & Indiv-Mx-LSTM & MX-LSTM   & TK         & TK + OCC \\ \hline
% Univ     & 0.53/1.16     & 0.49/1.12 & \textbf{0.44//0.99} &          \\ \hline
% Zara1    & 0.63/1.37     & 0.59/1.31 & \textbf{0.31/0.69}  &          \\ \hline
% Zara2    & 0.72/1.56     & 0.35/0.79 & \textbf{0.25/0.56}  &          \\ \hline
% \end{tabular}
% }
% \end{table}

\begin{table}[h]
  \centering
  \caption{Mean Average Displacement (MAD) error when changing the observation interval. Forecasting horizon is kept constant at 12 frames. \todo{Irtiza: calculate for the lstmon sgan dt}
  \label{table:table3Ab}
  
    \begin{tabular}{|l|l||l|l|}
    \hline
    Dataset & Prediction interval & Vanilla LSTM & TF-class (epoch 40)\\
    \hline \hline
    \multirow{3}{*}{\vspace{-1em}\textbf{Eth}} &
    \textbf{Obs = 8} & 0.61 / 1.20 & 1.01 /2.13\\
    \cline{2-4}
    &\textbf{Obs = 12} & 0.58 / 1.16 & na\\
    \cline{2-4}
    & \textbf{Obs = 16} & 0.59 / 1.18 & 0.97 / 1.92\\
    
    \hline \hline
    \multirow{3}{*}{\vspace{-1em}\textbf{Hotel}} &
    \textbf{Obs = 8} &  0.53 / 1.13 & 0.3 / 0.55\\
    \cline{2-4}
    & \textbf{Obs = 12} & 0.36 / 0.73 &  na \\
    \cline{2-4}
    & \textbf{Obs = 16} & 0.29 / 0.55 & 0.20 / 0.35\\
  
    \hline \hline
    \multirow{3}{*}{\vspace{-1em}\textbf{Ucy-univ}} &
    \textbf{Obs = 8} & 0.57 / 1.18 & 0.57 / 1.23\\
    \cline{2-4}
    &\textbf{Obs = 12} & 0.55 / 1.23 & na \\
    \cline{2-4}
    & \textbf{Obs = 16} & 0.53 / 1.19 & \\ 0.68 / 1.4
    \cline{2-4}
    \hline \hline
    \multirow{3}{*}{\vspace{-1 em}\textbf{Zara1}} &
    \textbf{Obs = 8} & 0.42 / 0.92 & 0.42 / 0.92\\
    \cline{2-4}
    &\textbf{Obs = 12} & 0.41 / 0.91 & na \\
    \cline{2-4}
    & \textbf{Obs = 16} & 0.41 / 0.92 & 0.43 / 0.98\\
    \cline{2-4}
    \hline \hline
    \multirow{4}{*}{\vspace{-1 em}\textbf{Zara2}} &
    \textbf{Obs = 8} & 0.35 / 0.78 & 0.33 / 0.74\\
    \cline{2-4}
    &\textbf{Obs = 12} & 0.32 / 0.72 & na \\
    \cline{2-4}
    & \textbf{Obs = 16} & 0.29 / 0.68 &  0.27/0.58\\
    \cline{2-4}

     \hline
    \end{tabular}
  
\end{table}
